# Supplementary material for: Topologically Directed Simulations Reveal the Impact of Geometric Constraints on Knotted Proteins
Source: arXiv:2504.12659 ancillary file (2025-04-17)
Supplement: Supplementary file 1 [file Supplementary_information.pdf]

# TOPOLOGICALLY DIRECTED SIMULATIONS REVEAL THE IMPACT OF GEOMETRIC CONSTRAINTS ON KNOTTED PROTEINS: SUPPLEMENTARY INFORMATION

AGNESE BARBENSI, ALEXANDER R. KLOTZ, DIMOS GKOUNTAROULIS

## 1. Molecular Dynamics Simulations

We simulate polymer knots with $N$ monomers using a commonly-used model, and our descriptions bear similarity to previous descriptions of these methods including our own. Polymers are comprised of beads of diameter $\sigma$ (which sets the lengthscale of the system) at position $\mathbf{r}_i(t)$, connected by springs to their two neighbors. A finitely-extensible nonlinear elastic (FENE) spring potential with a maximum extension of $1.5\sigma$ is used. Excluded volume interactions between beads are enforced by a truncated Lennard-Jones repulsive potential that applies when the centers of mass of two beads are closer than $1.122\sigma$. The relatively short range of distances between the excluded volume of the beads and maximum extension of the springs ensures that strands do not cross and the link topology is preserved. Bending rigidity is imposed by a Kratky-Porod potential depending on the cosine of the angle between three successive beads. The strength of this potential sets the persistence length of the polymer. The entire contribution to the energy of a bead is:

$$U_{\text{tot}} = U_{\text{spr}} + U_{\text{ev}} + U_{\text{bend}}\,. \tag{1}$$

The excluded volume interaction takes the form:

$$U_{\text{ev}} = \begin{cases} 4\epsilon\left[\left(\frac{\sigma}{r}\right)^{12} - \left(\frac{\sigma}{r}\right)^{6} + \frac{1}{4}\right] & \text{if } r \leq 2^{1/6}\sigma \\ 0 & \text{otherwise,} \end{cases} \tag{2}$$

where $\epsilon$ sets the energy scale of the repulsive interactions. The spring force is parameterized as:

$$U_{\text{spr}} = \begin{cases} -\frac{1}{2}\left(\kappa\frac{\epsilon}{\sigma^2}\right) R_{\max}\log\left|1 - \left(\frac{r}{R_{\max}}\right)^2\right|, & \text{if } r \leq R_{\max} \\ \infty & \text{otherwise,} \end{cases} \tag{3}$$

where $\kappa$ is 30 and sets the spring constant in units of $\epsilon/\sigma^2$, and $R_{\max} = 1.5\sigma$ is the maximum separation of the springs. The bending potential takes the form:

$$U_{\text{bend}} = \frac{\ell_p}{\sigma} kT(1 - \cos\theta)\,. \tag{4}$$

The dimensionless ratio of the persistence length $\ell_p$ to the bead diameter is $\ell_p/\sigma = 10$ in this work. The time evolution of the $i^{\text{th}}$ bead is determined by the Langevin equation:

$$m\ddot{\mathbf{r}}_i(t) = -\gamma\dot{\mathbf{r}}_i(t) - \nabla_{\mathbf{r}_i} U_{\text{tot}} + \sqrt{2kT\gamma}\,\eta(\mathbf{t})\,. \tag{5}$$

Here, $\gamma$ is the drag coefficient on a single bead, $kT$ is the thermal energy scale, $\eta$ is a delta-correlated normal random variable, i.e. $\langle \eta_i(t)\eta_j(t')\rangle = \delta_{ij}\delta(t-t')$, and an overdot represents a time derivative. The final term provides a random force that emulates Brownian motion in a manner consistent with the fluctuation-dissipation theorem. These equations of motion are solved by *LAMMPS* [1], which iterates the system forward in time using the Velocity Verlet algorithm.

The system is non-dimensionalized with $\sigma$, $\gamma$, $m$, $kT$ and $\epsilon$ taking values of 1, which defines a timescale $\tau_{LJ} = \sigma\sqrt{m/\epsilon}$. We iterate the simulation with a timestep of 0.001 $\tau$.

## 2. Other results: unoptimised growing model

The trajectories used to generate these results are available in the `unoptimised_growing` folder in our online repository: `https://zenodo.org/records/15220263`.

## References

[1] Thompson, Aidan P., et al. "LAMMPS-a flexible simulation tool for particle-based materials modeling at the atomic, meso, and continuum scales." Computer physics communications 271 (2022): 108171.

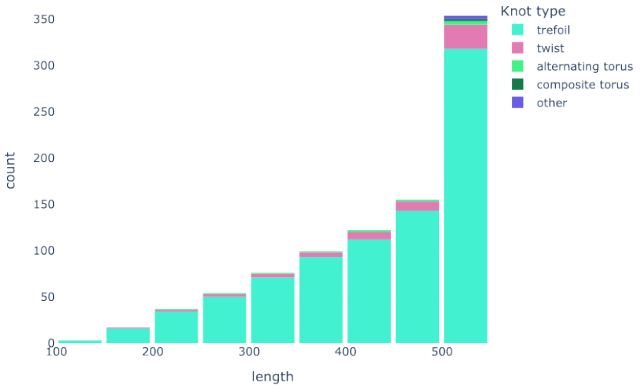


FIGURE 1. **Unbiased walks** Kymographs of knot formation during unoptimised walk growth, showing the fraction of different knot types in a population of 10,000 walks as a function of length.

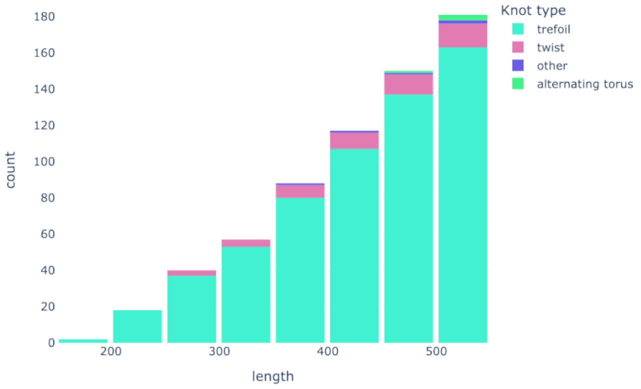


FIGURE 2. **No-helices protein-like walks** Kymographs of knot formation during unoptimised walk growth, showing the fraction of different knot types in a population of 10,000 walks as a function of length.

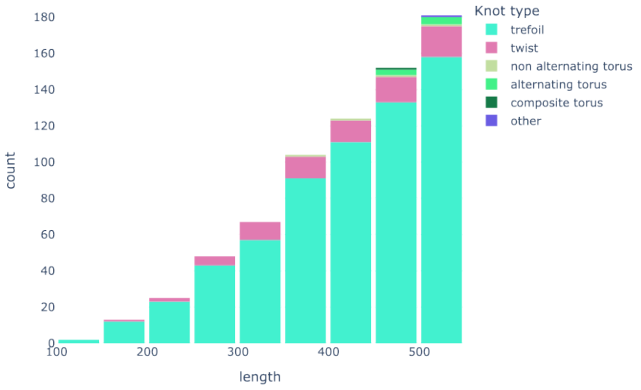


Figure 3. **Protein-like walks** Kymographs of knot formation during unoptimised walk growth, showing the fraction of different knot types in a population of 10,000 walks as a function of length.

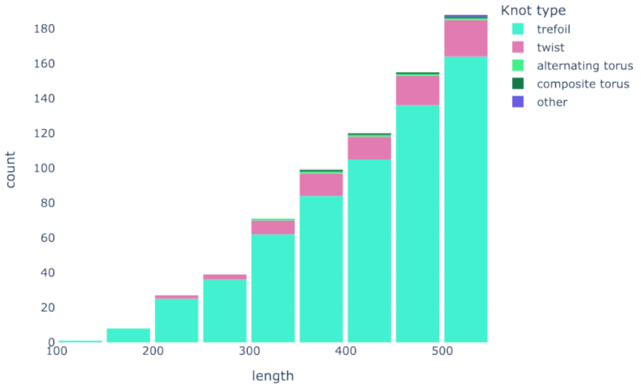


Figure 4. **Only-helices protein-like walks** Kymographs of knot formation during unoptimised walk growth, showing the fraction of different knot types in a population of 10,000 walks as a function of length.
